# Supplementary material for: REALM: Real-Time Estimates of Assistance for Learned Models in Human-Robot Interaction
Source: arXiv:2504.09243 source file (2025-04-12)
Supplement: Supplementary file 1 [file 06_appendix.tex]

\section{Expressions for Differential Entropy}
Our approach for estimating the value of assistance mechanisms requires specifying the post-intervention differential entropy for each mechanism. Here we provide more detail of the analytical differential entropy expressions for the teleoperation mechanism and the upper bound (i.e., $h_\textrm{max}$) used in calculating the mechanism likelihood.

\textbf{Teleoperation Entropy--}
Assuming the noisily optimal model, we can model the probability of action selection according to the differential entropy of a multivariate Gaussian distribution:
\begin{equation}
h(\mathcal{A}_t \mid m_{r}) \coloneq \frac{1}{2} \ln  \bigl\{ (2\pi e)^{n_a} |\Sigma_h | \bigr\} 
\end{equation}
where $n_a$ is the size of the action space and $\Sigma_h$ is the human's optimality (in the form of a covariance matrix). Under the simplifying assumption that the action variables are independent and with the same variance (i.e., derived from $\beta$), we can define the covariance matrix and further reduce the analytical expression to arrive at the expression presented in the technical overview:
\begin{align}
\Sigma_h &\coloneq \beta^{-1}\mathbf{I}_{n_a} \\
|\Sigma_h| &= \beta^{-n_a} \\
h(\mathcal{A}_t \mid m_{r}) &\coloneq \frac{1}{2} \ln  \bigl\{ (2\pi e)^{n_a} \beta^{-n_a} \bigr\} \\
&= \frac{1}{2}\ln (\beta^{-n_a})+\frac{1}{2}\ln \bigl\{ (2\pi e)^{n_a} \bigr\} \\
&= \frac{1}{2}\ln (\beta^{-n_a})+\frac{n_a}{2}\ln \bigl\{ (2\pi e) \bigr\} \\
&= \frac{1}{2}(\ln (\beta^{-n_a})+\frac{n_a}{2}\left(\ln(e)+\ln(2\pi)\right) \\
&= \frac{1}{2}(\ln (\beta^{-n_a})+\frac{n_a}{2}\left(1+\ln(2\pi)\right)
\end{align}

To provide a more intuitive understanding, $\beta$ corresponds to the inverse of the Gaussian distribution variance. For very low values of $\beta$, varied actions will have similar likelihoods. As $\beta$ increases and becomes large, only actions close to the optimal action are considered likely. In our experimental settings, all synthetic data was injected with Gaussian noise corresponding to a standard deviation of 0.001 (i.e., $\beta=1/(0.001)^2 = 1e6$). For simplicity, we assume the variance per action dimension is the same. However, this may not be realized in practice. For settings where this assumption is impractical, it is a trivial augmentation to the entropy formulation to assign different values to different dimensions. Furthermore, the assumption that error in the action variables is independent is for convenience. In cases where the error covariance can be estimated/measured and there are strong correlations (e.g., off-diagonal entries), the entropy can be calculated directly using the determinant of the covariance matrix (rather than the simplified expression for a diagonal matrix). We posit that it may be difficult to estimate such a human error term, and thus, use the simplified expression (which requires only a single parameter) in our implementation. Finally, it is also possible to compute the entropy estimates over normalized action spaces (though this can also cause non-meaningful variation to be amplified).

\textbf{Upper Bound from Data--}
To convert the differential entropy (which is unbounded) to a likelihood, our approach is to leverage upper and lower bounds on the entropy to convert the value to a positive range. As described in the paper, the upper bound for the entropy (i.e., most uncertainty) is defined as a uniform distribution over the range of possible action values from the robot policy. In our work, we have access to the training data and can directly compute the maximum and minimums over the action space. It is worth noting that actions can occur outside of the range (i.e., the Diffusion model can select an action outside of the training data), however, in practice, this uniform range of actions is very conservative in terms of entropy (i.e., it is incredibly unlikely the Diffusion model samples would compute a wider spread). If the training data is not available, the range of actions can be estimated through sampling or domain knowledge. To define the upper bound, we start with the definition of differential and substitute in the uniform distribution over action variables:
\begin{align}
p(\mathcal{A}_t) &\coloneq \prod \limits_{i}^{n_a} \frac{1}{\textbf{a}_{i,\textrm{max}} - \textbf{a}_{i,\textrm{min}}} \\
h(\mathcal{A}_t) &= \mathbb{E}[-log\left(p(\mathcal{A}_t)\right)] \\
h_{\textrm{max}}(\mathcal{A}_t) & \coloneq \mathbb{E}[-log\left(\prod \limits_{i}^{n_a} \frac{1}{\textbf{a}_{i,\textrm{max}} - \textbf{a}_{i,\textrm{min}}}\right)] \\
& = \mathbb{E}[log\left(\prod \limits_{i}^{n_a} (\textbf{a}_{i,\textrm{max}} - \textbf{a}_{i,\textrm{min}})\right)] \\
&= log\left(\prod \limits_{i}^{n_a} (\textbf{a}_{i,\textrm{max}} - \textbf{a}_{i,\textrm{min}})\right)
\end{align}
